# Supplementary material for: XC-Cache: Cross-Attending to Cached Context for Efficient LLM Inference
Source: arXiv:2404.15420 source file (2024-11-01)
Supplement: Supplementary file 5 [file appendix_hyperparameters.tex]

\vskip0.5cm

\section{Training hyperparameters}
\textbf{\label{sec:app-hyperparams}}

The main training hyperparameters used for \ourmodel{} are reported in Table~\ref{tab:hyperparams}.

\begin{table}[ht]
\small
\centering
\begin{tabular}{lc}
\toprule
Optimizer                                 & \textsc{AdamW}                 \\
Base learning rate                        & 0.0002                \\
Learning rate warmup steps                & 2,500                  \\
Maximum gradient norm                     & 1                     \\
Batch size                                & 256                   \\
Adam $\beta_1$                            & 0.9                   \\
Adam $\beta_2$                            & 0.95                  \\
Adam $\epsilon$                           & 0.000001              \\
Weight decay                              & 0.001                 \\
Cross-attention bias                      & False                 \\
Cross-attention dropout probability       & 0.2                   \\
Cross-attention final layer               & True                  \\
Cross-attention hidden size               & 2,048                 \\
Number of Cross-attention layers          & 5                     \\
Cross-attention layer skips               & 6                     \\
Cross-attention number of attention heads & 32                    \\
Cross-attention number of key value heads & 32                    \\
Numerical precision                       & 16-bit (BF16)         \\
Number of training steps                  & 40,000                \\ \bottomrule
\end{tabular}
\caption{Training hyperparameters for \ourmodel{}.}
\label{tab:hyperparams}
\end{table}
